# Supplementary material for: M22: A Communication-Efficient Algorithm for Federated Learning Inspired by Rate-Distortion
Source: arXiv:2301.09269 source file (2023-01-23)
Supplement: Supplementary file 1 [file appendix.tex]

%\comment{model details should be in appendix}

%
\begin{table}[t]
\vspace{0.5cm}
\footnotesize
    \centering
        \caption{A summary of the model layers of the CNN in Sec. \ref{sec:DNN training}. }
    \label{tab:cnn_model}
\begin{tabular}{|c|c|c|}
\hline
Layer (Type)      & Output Shape    & Param No.            \\ \hline
conv2d (Conv2D)     & (None, 32, 32, 32)   & 896      \\ (\emph{top layer, \#6}) & & \\ \hline
batch\_normalization        &     (None, 32, 32, 32)         & 128                                      \\ \hline
conv2d\_1 (Conv2D)     & (None, 32, 32, 32)   & 9248        \\ \hline
batch\_normalization\_1       &   (None, 32, 32, 32)           & 128                                           \\ \hline
max\_pooling2d (MaxPooling2D)     & (None, 16, 16, 32)   & 0        \\ \hline
dropout (Dropout)     &   (None, 16, 16, 32)          & 0                                          \\ \hline
conv2d\_2 (Conv2D) & (None, 16, 16, 64)          & 18496 \\\hline
batch\_normalization\_2 & (None, 16, 16, 64) & 256 \\\hline
conv2d\_3 (Conv2D) & (None, 16, 16, 64) & 36928\\\hline
batch\_normalization\_3 & (None, 16, 16, 64) & 256\\\hline
max\_pooling2d\_1 & (None, 8, 8, 64) & 0 \\\hline
dropout\_1 (Dropout)  & (None, 8, 8, 64) & 0 \\\hline
conv2d\_4 (Conv2D)   & (None, 8, 8, 128) & 73856\\ (\emph{middle layer, \#24}) & & \\\hline
batch\_normalization\_4 & (None, 8, 8, 128) & 512\\\hline
conv2d\_5 (Conv2D) &  (None, 8, 8, 128) & 147584\\\hline
batch\_normalization\_5 & (None, 8, 8, 128) & 512\\\hline
max\_pooling2d\_2 & (None, 4, 4, 128) & 0\\\hline
dropout\_2 (Dropout) & (None, 4, 4, 128) & 0\\\hline
flatten (Flatten) & (None, 2048) & 0\\\hline
dense (Dense) & (None,128) & 262272\\\hline
batch\_normalization\_6 & (None, 128) & 512 \\\hline
dropout\_3 (Dropout) & (None,128) & 0 \\\hline
dense\_1 (Dense)  & (None,10) & 1290\\ (\emph{bottom layer, \#42}) & & \\\hline
\end{tabular}
% \vspace{-0.5cm}
\end{table}

\begin{table}[t]
\vspace{0.5cm}
\footnotesize
    \centering
        \caption{A summary of the model layers of the ResNet18 in Sec. \ref{sec:DNN training}. }
    \label{tab:res18_model}
\begin{tabular}{|c|c|c|}
\hline
Layer (Type)      & Output Shape    & Param No.            \\ \hline
conv2d\_1 (Conv2D)     & (None, 16, 16, 64)   & 9408      \\ \hline
batch\_normalization\_1     &(None, 16, 16, 64)     & 128   \\ \hline
relu\_1    &(None, 16, 16, 64)     &0  \\ \hline
max\_pooling2d\_1      &(None, 8, 8, 64)     &0  \\  \hline
basic\_block\_1  \begin{tabular}{@{}l@{}}
                   conv2d\_2\\
                   batch\_normalization\_2\\
                   relu\_2\\
                   con2d\_3\\
                   batch\_normalization\_3\\
                   relu\_3\\
                 \end{tabular}      
                 
                 &\begin{tabular}{@{}l@{}}
                   (None, 8, 8, 64)\\
                   (None, 8, 8, 64)\\
                   (None, 8, 8, 64)\\
                   (None, 8, 8, 64)\\
                   (None, 8, 8, 64)\\
                   (None, 8, 8, 64)\\
                 \end{tabular}    
                 
                 &\begin{tabular}{@{}l@{}}
                   36864\\
                   128\\
                   0\\
                   36864\\
                   128\\
                   0\\
                 \end{tabular}  \\  \hline
basic\_block\_2     &(None, 8, 8, 64)   &73984  \\  \hline
basic\_block\_3     &(None, 4, 4, 128)   &230144  \\  \hline
basic\_block\_4     &(None, 4, 4, 128)   &295424  \\  \hline
basic\_block\_5     &(None, 2, 2, 256)   &919040  \\  \hline
basic\_block\_6     &(None, 2, 2, 256)   &1180672  \\  \hline
basic\_block\_7     &(None, 1, 1, 512)   &3673088  \\  \hline
basic\_block\_8     &(None, 1, 1, 512)   &4720640  \\  \hline
adaptive\_avg\_pool2d     &(None, 1, 1, 512)   &0  \\  \hline
dense\_1 (Dense)    &(None, 10) &5130   \\ \hline

\end{tabular}
% \vspace{-0.5cm}
\end{table}

\begin{table}[t]
\vspace{0.5cm}
\footnotesize
    \centering
        \caption{A summary of the model layers of the VGG16 in Sec. \ref{sec:DNN training}. }
    \label{tab:vgg16_model}
\begin{tabular}{|c|c|c|}
\hline
Layer (Type)      & Output Shape    & Param No.            \\ \hline
conv2d\_1 (Conv2D)     & (None, 32, 32, 64)   & 1792      \\ \hline
conv2d\_2 (Conv2D)     & (None, 32, 32, 64)   & 36928      \\ \hline
max\_pooling2d\_1      & (None, 16, 16, 64)     &0  \\  \hline
conv2d\_3 (Conv2D)     & (None, 16, 16, 128)   & 73856      \\ \hline
conv2d\_4 (Conv2D)     & (None, 16, 16, 128)   & 147584      \\ \hline
max\_pooling2d\_2      & (None, 8, 8, 128)     &0  \\  \hline
conv2d\_5 (Conv2D)     & (None, 8, 8, 256)   & 295168      \\ \hline
conv2d\_6 (Conv2D)     & (None, 8, 8, 256)   & 590080      \\ \hline
conv2d\_7 (Conv2D)     & (None, 8, 8, 256)   & 590080      \\ \hline
max\_pooling2d\_3      & (None, 4, 4, 256)     &0  \\  \hline
conv2d\_8 (Conv2D)     & (None, 4, 4, 512)   & 1180160      \\ \hline
conv2d\_9 (Conv2D)     & (None, 4, 4, 512)   & 2359808      \\ \hline
conv2d\_10 (Conv2D)    & (None, 4, 4, 512)   & 2359808      \\ \hline
max\_pooling2d\_4      & (None, 2, 2, 512)     &0  \\  \hline
conv2d\_11 (Conv2D)     & (None, 2, 2, 512)   & 2359808      \\ \hline
conv2d\_12 (Conv2D)     & (None, 2, 2, 512)   & 2359808      \\ \hline
conv2d\_13 (Conv2D)    & (None, 2, 2, 512)   & 2359808      \\ \hline
max\_pooling2d\_5      & (None, 1, 1, 512)     &0  \\  \hline
flatten               & (None, 512)         &0      \\ \hline
dense\_1              & (None, 4096)        &2101248    \\ \hline
dense\_2              & (None, 4096)        &16781312   \\ \hline
dense\_3              & (None, 10)          &40970      \\ \hline

\end{tabular}
% \vspace{-0.5cm}
\end{table}
